# Supplementary material for: Toward Long-Term and Archivable Reproducibility
Source: arXiv:2006.03018 source file (2022-05-09)
Supplement: Supplementary file 1 [file appendix-necessity.tex]

%% Appendix on reviewing the necessity for reproducible research
%% papers. This file is loaded by the project's 'paper.tex' or
%% 'tex/src/supplement.tex', it should not be run independently.
%
%% Copyright (C) 2020-2022 Mohammad Akhlaghi <mohammad@akhlaghi.org>
%% Copyright (C) 2021-2022 Raúl Infante-Sainz <infantesainz@gmail.com>
%
%% This file is free software: you can redistribute it and/or modify it
%% under the terms of the GNU General Public License as published by the
%% Free Software Foundation, either version 3 of the License, or (at your
%% option) any later version.
%
%% This file is distributed in the hope that it will be useful, but WITHOUT
%% ANY WARRANTY; without even the implied warranty of MERCHANTABILITY or
%% FITNESS FOR A PARTICULAR PURPOSE.  See the GNU General Public License
%% for more details. See <http://www.gnu.org/licenses/>.

\section{Necessity for reproducible research\\(not part of journal article; introductory review for non-specialists)}
\label{appendix:necessity}
The increasing volume and complexity of data analysis has been highly productive, giving rise to a new branch of ``Big Data'' in many fields of the sciences and industry.
However, given its inherent complexity, the mere results are barely useful alone.
Questions such as these commonly follow any such result:
What inputs were used?
What operations were done on those inputs? How were the configurations or training data chosen?
How did the quantitative results get visualized into the final demonstration plots, figures, or narrative/qualitative interpretation?
Could there be a bias in the visualization?
See Figure \ref{fig:questions} for a more detailed visual representation of such questions for various stages of the workflow.

In data science and database management, this type of metadata is commonly known as \emph{data provenance} or \emph{data lineage}.
Data lineage is being increasingly demanded for integrity checking from both the scientific, industrial, and legal domains.
Notable examples in each domain are respectively the ``Reproducibility crisis'' in the sciences that was reported by \emph{Nature} after a large survey \citeappendix{baker16}, and the General Data Protection Regulation (GDPR) by the European Parliament and the California Consumer Privacy Act (CCPA), implemented in 2018 and 2020, respectively.
The former argues that reproducibility (as a test on sufficiently conveying the data lineage) is necessary for other scientists to study, check and build-upon each other's work.
The latter requires the data-intensive industry to give individual users control over their data, effectively requiring thorough management and knowledge of the data lineage.
Besides regulation and integrity checks, having robust data governance (management of data lineage) in a project can be very productive: it enables easy debugging, experimentation on alternative methods, or optimization of the workflow.

In the sciences, the results of a project's analysis are published as scientific papers, which have traditionally been the primary conveyor of the lineage of the results: usually in narrative form, especially within the ``Methods'' section of the paper.
From our own experience, this section is often that which is the most intensively discussed during peer review and conference presentations, showing its importance.
After all, a result is defined as ``scientific'' based on its \emph{method} (the ``scientific method''), or lineage in data-science terminology.
In industry, however, data governance is usually kept as a trade secret and is not published openly or widely scrutinized.
Therefore, the main practical focus here will be on the scientific front, which has traditionally been more open to the publication of methods and anonymous peer scrutiny.

\begin{figure*}[t]
  \begin{center}
    \includetikz{figure-project-outline}{width=\linewidth}
  \end{center}
  \caption{\label{fig:questions}Graph of a generic project's workflow (connected through arrows), highlighting the various issues and questions on each step.
    The green boxes with sharp edges are inputs and the blue boxes with rounded corners are the intermediate or final outputs.
    The red boxes with dashed edges highlight the main questions at various stages in the work chain.
    The orange box, surrounding the software download and build phases, lists some commonly recognized solutions to the questions in it; for more discussion, see Appendix \ref{appendix:independentenvironment}.
  }
\end{figure*}

The traditional format of a scientific paper has been very successful in conveying the method and the results during recent centuries.
However, the complexity mentioned above has made it impossible to describe all the analytical steps of most modern projects to a sufficient level of detail.
Citing this difficulty, many authors limit themselves to describing the very high-level generalities of their analysis, while even the most basic calculations (such as the mean of a distribution) can depend on the software implementation.

Due to the complexity of modern scientific analysis, a small deviation in some of the different steps involved can lead to significant differences in the final result.
Publishing the precise codes of the analysis is the only guarantee of allowing this to be investigated.
For example, \citeappendix{smart18} describes how a 7-year old conflict in theoretical condensed matter physics was only identified after the different groups' codes were shared.
Nature is already a black box that we are trying hard to unlock and understand.
Not being able to experiment on the methods of other researchers is an artificial and self-imposed black box, wrapped over the original, and wasting much of researchers' time and energy.

A dramatic example showing the importance of sharing code is \citeappendix{miller06}, in which a mistaken flipping of a column was discovered, leading to the retraction of five papers in major journals, including \emph{Science}.
Ref.\/ \citeappendix{baggerly09} highlighted the inadequate narrative description of analysis in several papers and showed the prevalence of simple errors in published results, ultimately calling their work ``forensic bioinformatics''.
References \citeappendix{herndon14} and \citeappendix{horvath15} also reported similar situations and \citeappendix{ziemann16} concluded that one-fifth of papers with supplementary Microsoft Excel gene lists contain erroneous gene name conversions.
Such integrity checks are a critical component of the scientific method but are only possible with access to the data and codes and \emph{cannot be resolved from analyzing the published paper alone}.

The completeness of a paper's published metadata (or ``Methods'' section) can be measured by a simple question: given the same input datasets (supposedly on a third-party database like \href{http://zenodo.org}{zenodo.org}), can another researcher reproduce the same result automatically, without needing to contact the authors?
Several studies have attempted to answer this with different levels of detail.
For example, \citeappendix{allen18} found that roughly half of the papers in astrophysics do not even mention the names of any analysis software they have used, while \cite{menke20} found that the fraction of papers explicitly mentioning their software tools has greatly improved in medical journals over the last two decades.

Ref.\/ \citeappendix{ioannidis2009} attempted to reproduce 18 published results by two independent groups, but only fully succeeded in two of them and partially in six.
Ref.\/ \citeappendix{chang15} attempted to reproduce 67 papers in well-regarded economic journals with data and code: only 22 could be reproduced without contacting authors, and more than half could not be replicated at all.
Ref.\/ \citeappendix{stodden18} attempted to replicate the results of 204 scientific papers published in the journal Science \emph{after} that journal adopted a policy of publishing the data and code associated with the papers.
Even though the authors were contacted, the success rate was $26\%$.
Generally, this problem is unambiguously felt in the community: \citeappendix{baker16} surveyed 1574 researchers and found that only $3\%$ did not see a ``reproducibility crisis''.

This is not a new problem in the sciences: in 2011, Elsevier conducted an ``Executable Paper Grand Challenge'' \citeappendix{gabriel11}.
The proposed solutions were published in a special edition.
Some of them are reviewed in Appendix \ref{appendix:existingsolutions}, but most have not been continued since then.
In 2005, Ref.\/ \citeappendix{ioannidis05} argued that ``most claimed research findings are false''.
Even earlier, in the 1990s, Refs \cite{schwab2000}, \citeappendix{buckheit1995} and \cite{claerbout1992} described this same problem very eloquently and provided some of the solutions that they adopted.
While the situation has improved since the early 1990s, the problems mentioned in these papers will resonate strongly with the frustrations of today's scientists.
Even earlier yet, through his famous quartet, Anscombe \citeappendix{anscombe73} qualitatively showed how the distancing of researchers from the intricacies of algorithms and methods can lead to misinterpretation of the results.
One of the earliest such efforts we found was \citeappendix{roberts69}, who discussed conventions in FORTRAN programming and documentation to help in publishing research codes.

From a practical point of view, for those who publish the data lineage, a major problem is the fast-evolving and diverse software technologies and methodologies that are used by different teams in different epochs.
Ref.\/ \citeappendix{zhao12} describes it as ``workflow decay'' and recommends preserving these auxiliary resources.
But in the case of software, this is not as straightforward as for data: if preserved in binary form, the software can only be run on a certain operating system on particular hardware, and if kept as source code, its build dependencies and build configuration must also be preserved.
Ref.\/ \citeappendix{gronenschild12} specifically studies the effect of software version and environment and encourages researchers to not update their software environment.
However, this is not a practical solution because software updates are necessary, at least to fix bugs in the same research software.
Generally, the software is not a secular component of projects, where one software package can easily be swapped with another.
Projects are built around specific software technologies, and research in software methods and implementations is itself a vibrant research topic in many domains \citeappendix{dicosmo19}.
