# Supplementary material for: Toward Long-Term and Archivable Reproducibility
Source: arXiv:2006.03018 source file (2022-05-09)
Supplement: Supplementary file 2 [file supplement.tex]

%% The top-level file to build the separate supplement that contains the
%% appendices (to be published as a separate PDF file).
%
%% Copyright (C) 2020-2022 Mohammad Akhlaghi <mohammad@akhlaghi.org>
%% Copyright (C) 2020-2022 Boudewijn F. Roukema <boud@astro.uni.torun.pl>
%
%% This file is free software: you can redistribute it and/or modify it
%% under the terms of the GNU General Public License as published by the
%% Free Software Foundation, either version 3 of the License, or (at your
%% option) any later version.
%
%% This file is distributed in the hope that it will be useful, but WITHOUT
%% ANY WARRANTY; without even the implied warranty of MERCHANTABILITY or
%% FITNESS FOR A PARTICULAR PURPOSE.  See the GNU General Public License
%% for more details. See <http://www.gnu.org/licenses/>.
\documentclass[journal]{IEEEtran}

%% This is a convenience variable if you are using PGFPlots to build plots
%% within LaTeX. If you want to import PDF files for figures directly, you
%% can use the standard `\includegraphics' command. See the definition of
%% `\includetikz' in `tex/preamble-pgfplots.tex' for where the files are
%% assumed to be if you use `\includetikz' when `\makepdf' is not defined.

%% VALUES FROM ANALYSIS (NUMBERS AND STRINGS): this file is automatically
%% generated at the end of the processing and includes LaTeX macros
%% (defined with '\newcommand') for various processing outputs to be used
%% within the paper.
\input{tex/build/macros/project.tex}
\input{tex/src/preamble-maneage.tex}

%% Import the other necessary TeX files for this particular project.
\input{tex/src/preamble-project.tex}

%% Title and author names.
\title{\textsc{\LARGE Supplemental appendices for paper:}\\ \emph{\projecttitle}}
\author{
  Mohammad Akhlaghi,
  Ra\'ul Infante-Sainz,
  Boudewijn F. Roukema,
  Mohammadreza Khellat,\\
  David Valls-Gabaud,
  Roberto Baena-Gall\'e\\
  \footnotesize{Manuscript received June 5th, 2020; accepted April 7th, 2021; first published by CiSE April 13th, 2021}
}

%% The paper headers
\markboth{Computing in Science and Engineering, Vol. 23, Issue 3, Pages 82--91, 2021: \href{https://doi.org/10.1109/MCSE.2021.3072860}{DOI:10.1109/MCSE.2021.3072860}, arXiv:2006.03018, \href{https://doi.org/10.5281/zenodo.\projectzenodoid}{zenodo.\projectzenodoid}}%
{Akhlaghi \MakeLowercase{\textit{et al.}}: \projecttitle}

%% Start the paper.
\begin{document}

% make the title area
\maketitle

% For peer review papers, you can put extra information on the cover
% page as needed:
% \ifCLASSOPTIONpeerreview
% \begin{center} \bfseries EDICS Category: 3-BBND \end{center}
% \fi
%
% For peerreview papers, this IEEEtran command inserts a page break and
% creates the second title. It will be ignored for other modes.
\IEEEpeerreviewmaketitle

%% A short appendix describing this file.
\begin{abstract}
  This supplement contains appendices to the main body of Akhlaghi et al., published in CiSE (\href{https://doi.org/10.1109/MCSE.2021.3072860}{DOI:10.1109/MCSE.2021.3072860}, available as a preprint at \href{https://arxiv.org/abs/\projectarxivid}{\texttt{arXiv:\projectarxivid}} or \href{https://doi.org/10.5281/zenodo.\projectzenodoid}{\texttt{zenodo.\projectzenodoid}}).
  In the paper's main body we introduced criteria for longevity of reproducible workflow solutions and introduced a proof of concept that implements them, called Maneage (\emph{Man}aging data lin\emph{eage}).
  This supplement provides an in-depth literature review of previous methods and compares them and their lower-level tools in detail with our criteria and with the proof of concept presented in this work.
  Appendix \ref{appendix:existingtools} reviews the low-level tools that are used by many reproducible workflow solutions (including our proof of concept).
  Appendix \ref{appendix:existingsolutions} reviews many solutions that attempt(ed) reproducible management of workflows (including solutions that have stopped development, or worse, are no longer available online).
  To highlight the evolving landscape and its effects on longevity, Appendix \ref{appendix:existingsolutions}  discusses the solutions in historical order.
  Finally, in Appendix \ref{appendix:software} an automatically generated, exhaustive list of software used to build this project is included with the software versions indicated.
  This supplement was built from project commit \projectversion.
\end{abstract}

%% Import the appendices.
\appendices
\input{tex/src/appendix-existing-tools.tex}
\input{tex/src/appendix-existing-solutions.tex}
\input{tex/src/appendix-used-software.tex}

%% Bibliography.
\bibliographystyle{IEEEtran_openaccess}
\bibliography{IEEEabrv,references}

%% End the paper.
\end{document}
